# Supplementary material for: Bounded-error constrained state estimation of LTV systems in presence of sporadic measurements
Source: arXiv:2202.13900 source file (2023-09-14)
Supplement: Supplementary file 1 [file Appendix_propo_rank_pseudo-inv.tex]

\subsection{Proof of Proposition \ref{propo_pseudo-inv}}
\label{Appendix_propo_rank_pseudo-inv}
\eqref{eq_pseudo-inv-rec} can be obtained by applying Thm 1 and Thm 3 of \cite{Mey:73}.
