# Supplementary material for: Bounded-error constrained state estimation of LTV systems in presence of sporadic measurements
Source: arXiv:2202.13900 source file (2023-09-14)
Supplement: Supplementary file 2 [file Appendix_theo_meas_update_vol.tex]

\subsection{Proof of Theorem \ref{theo_meas_update_vol}}
\label{Appendix_theo_meas_update_vol}
Same proof as for Thm \ref{theo_meas_update} when using  Thm \ref{theo_beta_vol_min} instead of Thm \ref{theo_beta_sig_min}. 
\eqref{eq_correc-q}, where ${q}\kij{i}\eqg \rank(\Pki)$,  is obtained considering, from \eqref{eq_correc-P}, that  
\begin{align}
\Pki\eqg\Pkiii^{\frac{1}{2}}\big(I_n-\betak{i}{\bfbki\bfbki^\dag}\big)\Pkiii^{\frac{1}{2}}\nn
\end{align}
where $\bfbki=\Pkiii^{\frac{1}{2}}\fbki$ and $I_n-{\bfbki\bfbki^\dag}$ is the orthogonal projector onto the kernel of $\bfbki$, implying that
$\rank(\Pki)=\rank(\Pkiii)-1$ whenever $\betak{i}=1$ and $\rank(\Pki)=\rank(\Pkiii)$, otherwise.
